# Supplementary material for: UniVTG: Towards Unified Video-Language Temporal Grounding
Source: arXiv:2307.16715 source file (2023-08-18)
Supplement: Supplementary file 1 [file supp.tex]

\documentclass[10pt,twocolumn,letterpaper]{article}

\usepackage{iccv}
\usepackage{times}
\usepackage{epsfig}
\usepackage{graphicx}
\usepackage{amsmath}
\usepackage{amssymb}
\usepackage{marvosym}
\usepackage{lipsum}
\usepackage{float}
\usepackage{multirow}
\usepackage{subfigure}
\usepackage{tikz,pgfplots}
\usepackage{amsmath}
\usepackage{amssymb}
\usepackage{booktabs}
\usepackage{graphicx}
\usepackage{multirow}
\usepackage{nccfoots}
\usepackage{tabularx}
\usepackage{bbm}
\usepackage{comment}
\usepackage{threeparttable}
\usepackage{enumitem}
\usepackage{caption}
\pagestyle{empty}  % remove page number;
% \usepackage[dvipsnames]{xcolor}
% https://www.overleaf.com/learn/latex/Using_colours_in_LaTeX
\usepackage{color, colortbl}
\usepackage{stfloats}
\usepackage{pifont}
\usepackage{footnote}

\definecolor{citecolor}{HTML}{0071bc}
\usepackage[pagebackref=false,breaklinks=true,letterpaper=true,colorlinks,citecolor=citecolor,bookmarks=false]{hyperref}
\usepackage[capitalize]{cleveref}
\crefname{section}{Sec.}{Secs.}
\Crefname{section}{Section}{Sections}
\Crefname{table}{Table}{Tables}
\crefname{table}{Tab.}{Tabs.}

\definecolor{citecolor}{HTML}{0071bc}
\definecolor{color_ao}{gray}{0.5}
\definecolor{color_our}{rgb}{0.66,0.82,0.56}
\definecolor{color_pre}{rgb}{0.52,0.59,0.69}
\definecolor{Gray}{gray}{0.9}
\definecolor{LighterGray}{gray}{0.93}
\definecolor{LightGrayForTableRule}{gray}{0.92}
\definecolor{DarkGray}{gray}{0.5}
\definecolor{Black}{rgb}{0.0, 0.0, 0.0}
\definecolor{NiceBlue}{rgb}{0.11764705882352941, 0.5647058823529412, 1.0}
\definecolor{NiceGreen}{rgb}{0.0, 0.5, 0.0}
\usepackage{pgfkeys}
	\def\addlegendimage{\csname pgfplots@addlegendimage\endcsname}

\iccvfinalcopy % 
 % *** Enter the ICCV Paper ID here

\definecolor{Yellow}{RGB}{255, 242, 204}
\definecolor{Cyan}{RGB}{202, 242, 204}
% Pages are numbered in submission mode, and unnumbered in camera-ready
% \ificcvfinal\pagestyle{empty}\fi

\begin{document}

\newcommand{\vtg}{VTG}
\newcommand{\vlp}{VLP}
\newcommand{\VTG}{Video Temporal Grounding}
\newcommand{\VLP}{Vision-Language Pretraining}
\newcommand{\VLTG}{Video-Language Temporal Grounding}
\newcommand{\our}{{UniVTG}}
\newcommand{\unit}{clip}

\newcommand{\mr}{moment retrieval}
\newcommand{\hl}{highlight detection}
\newcommand{\vsum}{video summarization}
\newcommand{\tal}{temporal action localization}

\newcommand{\MR}{Moment Retrieval}
\newcommand{\HL}{Highlight Detection}
\newcommand{\VS}{Video Summarization}
\newcommand{\TAL}{Temporal Action Localization}

\newcommand{\data}{label}
\newcommand{\Interval}{Interval-wise}
\newcommand{\Curve}{Curve-wise}
\newcommand{\Point}{Point-wise}
\newcommand{\interval}{interval}
\newcommand{\curve}{curve}
\newcommand{\point}{point}
\newcommand{\intervall}{interval-level}
\newcommand{\curvel}{curve-level}
\newcommand{\pointl}{point-level}

\newcommand{\format}{unified \data~format}
\newcommand{\Format}{Unified \data~format}

\newcommand{\ind}{foreground indicator}
\newcommand{\bdy}{boundary offsets}
\newcommand{\sal}{saliency score}

\newcommand{\detr}{Moment-DETR}
\newcommand{\iv}{IntentVizor}

\newcommand{\qv}{QVHighlights}
\newcommand{\charades}{Charades-STA}
\newcommand{\anet}{Activitynet Captions}
\newcommand{\ego}{Ego4D}
\newcommand{\youtube}{YouTube Highlights}
\newcommand{\tvsum}{TVSum}
\newcommand{\qfvs}{QFVS}
\newcommand{\tacos}{TACoS}
\newcommand{\nlq}{NLQ}
\newcommand{\NLQ}{Natural Language Queries}
\newcommand{\supp}{Supplementary}
\newcommand{\sota}{state-of-the-art}

% Remove page # from the first page of camera-ready.
\ificcvfinal\thispagestyle{empty}\fi

\input{ICCV/appendix}

{
\bibliographystyle{ieee_fullname}
\bibliography{main}
}

\end{document}
